# Supplementary material for: Supersymmetry production cross sections in pp collisions at sqrt{s} = 7 TeV
Source: arXiv:1206.2892 source file (2012-06-13)
Supplement: Supplementary file 1 [file appendix.tex]

\section{Appendix A: detailed cross section results using CMSSM plane}

Should we refer to the twiki here or we put it in sections 4 and 5 and remove the appendix?

%In this appendix we report a more detailed breakdown of the cross sections  
%which have been presented in the text. In particular, we explicitly present
%all NLO cross-sections as well as NLO+NLL determined with the different PDF sets
%in the CMSSM plane. The central values and the combined total errors on the cross section 

%are obtained using envolope of scale and PDF variations for each of the 10 sub-processes.
%The breakdown of these cross sections can be obtained using reference~\cite{combined7TeV}.
%The results are given for $\tan\beta =10, A_{0} = 0, \mu > 0$ and $\tan\beta =40, A_{0} = -500, \mu > 0$ 
%in the $m_{0} - m_{1/2}$ plane.
